# Supplementary material for: Dimensionality Reduction for Sum-of-Distances Metric
Source: arXiv:1912.12003 source file (2021-06-24)
Supplement: Supplementary file 1 [file appendix_dense.tex]

\section{Omitted Proofs in \cref{sec:fastcomputation}}\label{sec:fast-dense}
% \fastlmawellcondbasiscomp*
\begin{proof}[Proof of \cref{lma:fast-well-cond-basis-comp}]
	To compute a well-conditioned basis for the matrix $A(I-P)R$, we first compute a $QW_1$ decomposition of the matrix $\Pi A(I-P)R$ for a $\Pi$ which is an $\ell_1$ subspace embedding. Then, $A(I-P)RW_1^{-1}$ is the required well conditioned basis. Given that $\Pi A$ is already computed, $\Pi A(I-P)R = \Pi A R - \Pi AP R = \Pi A R - \Pi A WW^TR$ can be computed in $O(d \cdot \poly(k/\epsilon))$ time. Now, $\Pi A(I-P)R$ is a small matrix and hence its $QW_1$ decomposition as well as $W_1^{-1}$ can be computed in time $\poly(k/\epsilon)$. Hence, the total time required to compute $W_1^{-1}$ is $O(d \cdot \poly(k/\epsilon))$.
\end{proof}
% \fastlmapartitionsumleveragescores*
%\subsection{}
\begin{proof}[Proof of \cref{lma:partitionapproxls}]
Sum of $\ell_1$ leverage scores of rows of $A(I-P)R$ in a partition $P_i$ is given by 
    \begin{equation}
        \sum_{j} \|(A[P_i](I-P_B)RW^{-1})_{j*}\|_1
    \end{equation}
    where $A(I-P)RW^{-1}$ is a well conditioned basis for the matrix $A(I-P_B)R$. We can re-write this as
    \begin{align*}
        \sum_{j} \|(A[P_i](I-P_B)RW^{-1})_{j*}\|_1 &= \sum_{j} \sum_{k} |(A[P_i](I-P_B)RW^{-1})_{jk}|\\
        &= \sum_{k}\sum_{j}|(A[P_i](I-P_B)RW^{-1})_{jk}|\\
        &= \sum_k \|(A[P_i](I-P_B)RW^{-1})_{*k}\|_1.
    \end{align*}

Now, a $1+\epsilon$ approximation to the $\ell_1$ norm of a column can be computed by pre-multiplying it by a Cauchy Matrix and then taking the median of absolute values of coordinates of the product. Using a Cauchy matrix with $\poly(k/\epsilon)\log(n)$ rows, the norms are preserved up to $1\pm 1/\poly(k/\epsilon)$ with  probability  $\ge 1 - 1/\poly(k/\epsilon)$. So, we can use the same $C$ matrix for all of the $\poly(k/\epsilon)$ columns and union bound the error probability over all the $\poly(k/\epsilon)$ columns of the matrix $A[P_i](I-P_B)RW^{-1}$ to get that the estimates of the $\ell_1$ norms are within $1 \pm \text{1}/{\poly(k/\epsilon)}$ of the actual values with probability at least $\ge 1 -1/\poly(k/\epsilon)$.
Given that $C_iA[P_i]$ has been computed, $1\pm \epsilon$ approximations for the $\ell_1$-norms of all columns of $A[P_i](I-P_B)RW^{-1}$ can be computed in $O(d \cdot \poly(k/\epsilon))$ time.

Thus, we approximate $\|(A[P_i](I-P_B)RW^{-1})_{*k}\|$ by $\text{median}(\text{abs}((C_iA[P_i](I-P_B)RW^{-1})_{*k}))$ for all the columns and hence can compute the approximate sum of $\ell_1$ leverage scores of rows in a partition.
\end{proof}
% \fastlmasucceedswithfewlight*
\begin{proof}[Proof of \cref{lma:fixed-light-rows}]
    Let $S$ be the random variable denoting the number of \emph{light} rows sampled by $\ell_1$ leverage score sampling. Let $\text{Succeeds}$ be the event that leverage score sampling succeeds. We have the following
    \begin{align*}
        \text{E}[S] &= \text{E}[S | \text{\textbf{Succeeds}}] \cdot \text{Pr}[\textbf{Succeeds}] + \text{E}[S | \neg\textbf{Succeeds}] \cdot \text{Pr}[\neg \textbf{Succeeds}]\\
        &\ge \text{E}[S | \textbf{Succeeds}] \cdot \text{Pr}[\textbf{Succeeds}]\\
    \end{align*}
    Hence, $\text{E}[S | \text{Succeeds}] \le \text{E}[S]/\text{Pr}[\text{Succeeds}] \le 2\text{E}[S]$.
    \begin{align}
        \text{Pr}[S \ge 10 \cdot \poly_1(k/\epsilon)  | \textbf{Succeeds}] & \le \text{E}[S|\textbf{Succeeds}]/(10 \cdot \poly_1(k/\epsilon) ) \nonumber \\
        &\le 2 \cdot \poly_1(k/\epsilon)/(10 \cdot \poly_1(k/\epsilon)) \nonumber \\
        &= 1/5
    \end{align}
Finally we have
\begin{align}
    &\text{Pr}[\textbf{Succeeds} | S \le 10 \cdot \poly_1(k/\epsilon) ]\\ 
    &= \frac{\text{Pr}[S \le 10 \cdot \poly_1(k/\epsilon)  | \textbf{Succeeds}] \cdot \text{Pr}[\textbf{Succeeds}]}{\text{Pr}[S \le 10 \cdot \poly_1(k/\epsilon) ]} \nonumber \\
    &\ge \text{Pr}[S \le 10 \cdot \poly_1(k/\epsilon)  | \textbf{Succeeds}] \cdot \text{Pr}[\textbf{Succeeds}]\nonumber \\
    &\ge \left(1 -\frac15\right) \cdot (1 - c) \qedhere
\end{align}
\end{proof}
\begin{proof}[Proof of \cref{lma:sampling-light-rows-fast}]
	For $P \in \calP_l$, let $\textnormal{act}(P)$ be the actual sum of probabilities of rows in $P$ and $\textnormal{approx}(P)$ be the approximation of $\textnormal{act}(P)$ computed as in \cref{lma:partitionapproxls}. So, we have that for all $P \in \calP_l$
	\begin{equation}
		\left(1 - \frac{1}{\beta p(k/\epsilon)^3}\right) \le \frac{\text{approx}(P)}{\text{act}(P)} \le \left(1 + \frac{1}{\beta p(k/\epsilon)^3}\right),
		\label{eqn:relating-actual-approx-sum}
	\end{equation}
	where $\beta \ge 10^3$. Consider the interval $[0,\sum_{P \in \calP_l}\text{approx}(P)]$ subdivided into intervals each of length $\text{approx}(P)$ for each $P$ in $\calP_l$. Now choose $r$ points uniformly at random in this interval. Consider each $P \in \calP_l$ which contains at least one of the $r$ $\ell_1$ leverage scores. There are at most $r$ such partitions and exact leverage scores are computed for at most $n/p(k/\epsilon)^8 \cdot r \le 10 \cdot n/p(k/\epsilon)^7$ rows as $r \le 10 \cdot p(k/\epsilon)$. Now further subdivide the interval corresponding to a \emph{light} partition into intervals proportional to the  probabilities of sampling the rows in those intervals. Then choose the rows corresponding to the sub-intervals that contain $r$ sampled points. Using the fact that $\text{approx}(P) \le 1/p(k/\epsilon)^5$ for $P \in \calP_l$ and assuming $\sum_{P \in \calP_l}\text{approx}(P) \ge 1$, we can show that no sub-interval contains more than $2$ sampled points with probability $\ge 1 - O(1/p(k/\epsilon)^3)$. We assume that the event that the $r$ sampled points correspond to $r$ distinct intervals holds, and add to our overall failure probability. 
	
	Let $p_i$ be the event that the $i$-th row is sampled by $\ell_1$ leverage score sampling for $i \in [n]$. Let $R \subseteq [n]$ be an arbitrary subset of $r$ \emph{light} rows sampled by $\ell_1$ leverage score sampling. We have that the probability that the set of \emph{light} rows sampled by leverage score sampling conditioned on leverage score sampling sampling $r$ \emph{light} rows is 
	\begin{equation*}
		\propto \prod_{i \in R}\left(\frac{p_i}{1-p_i}\right)
		= C\prod_{i \in R}\left(\frac{p_i}{1-p_i}\right),
	\end{equation*}
	where $C$ is a normalization constant.
	Using the fact that $p_i \le 1/p(k/\epsilon)^5$ and $|R| = r \le 10 \cdot p(k/\epsilon)$, we obtain that
	\begin{equation}
		\left(1 + \frac{1}{\Theta(p(k/\epsilon)^4)}\right)\prod_{i \in R}p_i \ge \prod_{i \in R}\left(\frac{p_i}{1-p_i}\right) \ge \prod_{i \in R}p_i.
	\end{equation}
The probability that the set of rows sampled by the sampling process described above is $R$ is 
\begin{equation*}
	\propto \prod_{i \in R}p_i \frac{\text{approx(part($i$))}}{\text{act(part($i$))}}
	= D\prod_{i \in R}p_i \frac{\text{approx(part($i$))}}{\text{act(part($i$))}},
\end{equation*}
where part($i$) denotes the $P \in \calP_l$ that contains $i$ and $D$ is a normalization constant. From \eqref{eqn:relating-actual-approx-sum}, we obtain that
\begin{equation}
1 - \frac{1}{\Theta(p(k/\epsilon)^2)} \le \prod_{i \in R} \frac{\text{approx(part($i$))}}{\text{act(part($i$))}} \le 1 + \frac{1}{\Theta(p(k/\epsilon)^2)}.
\end{equation}
From this we can conclude that the total variation distance between leverage score sampling conditioned on $r$ rows being sampled and the above sampling process is $\le 1/\Theta(p(k/\epsilon)^2)$. The running time arguments follow from the fact that only $O(nd/p(k/\epsilon)^7)$ leverage scores have to be calculated and that given all the matrices required, this can be done in $\tilde{O}(nd/p(k/\epsilon)^7 + (n+d)\poly(k/\epsilon))$.
\end{proof}
\begin{proof}[Proof of \cref{lma:best-sampling-matrix}]
Let $\mathcal{S}$ be a Cauchy matrix with $O(\log(n)/\epsilon)$ rows and $G$ be a random $\R^{d \times \log(n\poly(k/\epsilon))/\epsilon^2}$ random Gaussian matrix. With high probability $\|xG\|_2 = g(1 \pm \epsilon)\|xG\|_1$ for some constant $g$ for any $O(n \cdot \poly(k/\epsilon))$ vectors (Lemma 5.3 of \cite{doi:10.1002/cpa.21442}). Also note that $G$ preserves the 2-norm of any $O(n \cdot \poly(k/\epsilon))$  vectors with some scaling factor with high probability. We condition on the event that both the properties hold. Let $X_j$ be the projection matrix corresponding to the solution for the problem with the sampling matrix $S_j$. Given that $\mathcal{S}A$ is already computed, we can compute $\mathcal{S}A(I-P_B)X_jG - \mathcal{S}A(I-P_B)G$ in time $O(d \cdot \poly(k/\epsilon))$. We can then compute an approximation of the cost
\begin{align*}
    &\|A(I-P_B)X_j - A(I-P_B)\|_{1,2} \\
    &= \sum_{i}\|A_{i*}(I-P_B)X_j - A_{i*}(I-P_B)\|_2\\
    &= c(1 \pm \epsilon) \sum_{i} \|A_{i*}(I-P_B)X_jG - A_{i*}(I-P_B)G\|_2\\
    &\quad \text{(Conditioned on the event $G$ that it preserves the $2$-norm)}\\
    &= (c/g)(1 \pm \epsilon)^2 \sum_{i} \|A_{i*}(I-P_B)X_jG - A_{i*}(I-P_B)G\|_1\\
    &\quad \text{(Since, $\|\cdot\|_1$ and $\| \cdot \|_2$ are related as above)}\\
    &= (c/g)(1 \pm \epsilon)^2 \sum_{\text{columns}\ t} \|(A(I-P_B)X_jG - A(I-P_B)G)_{*t}\|_1\\
    &= (c/g)(1 \pm \epsilon)^2 \sum_{\text{columns}\ t} \text{med}(\text{abs}((\mathcal{S}A(I-P_B)X_jG - \mathcal{S}A(I-P_B)G)_{*t})).
\end{align*}
Here, $\text{med}(v)$ denotes the median absolute value among the coordinates of vector $v$. Thus we can compute the approximate cost of a solution given that $\mathcal{S}A$ has already been computed in time $O(d\log n \log d \poly(k/\epsilon))$, and hence can find the sampling matrix $S_j$ with cost at most $(1+O(\epsilon))$ times that of the best sampling matrix, in time $O(d\log n \log d \poly(k/\epsilon))$.
\end{proof}
\begin{proof}[Proof of \cref{thm:fastcomputeallmatrices}]
    All the matrices which are pre-multiplied with $A$ have $\poly(k/\epsilon)$ or $\log (n)/\epsilon$ rows. So, we can form a big matrix having at most $O(\poly((k + \log(n))/\epsilon))$ rows and $n$ columns. Let this matrix be called $\mathcal{P}$. Divide $\mathcal{P}$ into $n/d$ block matrices each having $d$ columns and divide $A$ into $n/d$ block matrices each having $d$ rows. Now, $\mathcal{P} \cdot A$ is the sum of $n/d$ product matrices $\mathcal{P}_i A^i$ where $\mathcal{P}_i$ is a $\poly((k + \log(n))/\epsilon) \times d$ matrix and $A^i$ is a $d \times d$ matrix. We can assume that $\poly((k + \log(n))/\epsilon) \le d^{0.1}$. Otherwise, we can just do the computation in $\poly((k + \log(n))/\epsilon)$ time for some polynomial and the results will still hold. Now, we can use a fast multiplication algorithm for rectangular matrices from \cite{coppersmith}, which runs in time $O(d^2\log^2(d)))$. So, all of the $n/d$ products can be computed in $O(nd\log(d)) + n\cdot\poly((k + \log(n))/\epsilon)$ time, and their sum can be computed in $O(d \cdot \poly(k/\epsilon))$ time.
\end{proof}
