# Supplementary material for: Dimensionality Reduction for Sum-of-Distances Metric
Source: arXiv:1912.12003 source file (2021-06-24)
Supplement: Supplementary file 2 [file appendix_pge2.tex]

\section{Sum of \texorpdfstring{$p^{\text{th}}$}{p} Powers of Euclidean Distance When \texorpdfstring{$p>2$}{p>2}}\label{sec:adaptivesample}
For clustering using $p<2$ we can use the non-adaptive algorithm in \cite{clarkson2015input} because we can compute $\ell_p$ leverage scores efficiently. However, for $p>2$, there is no oblivious subspace embedding so this technique cannot be adopted. In this section, we provide an adaptive algorithm that runs in time $O(\frac{1}{\epsilon^{2/p}}nd\poly(k/\epsilon))$, based on the adaptive sampling technique in \cite{deshpande2007sampling}.

	\begin{algorithm}[!ht]
			\DontPrintSemicolon
	    \SetKwInOut{Input}{Input}
	    \SetKwInOut{Output}{Output}
	    \SetKwData{Start}{start}
	    \SetKwData{End}{end}
		\caption{\textsc{SamplingSubspace}}
		\label{alg:samplingsubspace}
			\Input{ $A\in\R^{n\times d}$ with row vectors $a_1,\ldots, a_n$, $k>0$, a ``base'' approximate subspace projection $P_B\in\R^{d\times d}$ we have found so far, a problem parameter $k>0$, an approximately good projection $P_{\hat{X}}\in\R^{d\times d}$, accuracy $\epsilon>0$, approximation factor $K$ of $P_{\hat{X}}$.}
			\Output{ Subspace approximation $S\subseteq [n]$ of $O((\poly(k)/\epsilon)^p\cdot k^2/\epsilon\cdot\log(\poly(k)/\epsilon))$.}
			 Find subspace $V$ of dimension at least $k$ using \fref{alg:polykapprox} such that \;
				\begin{equation*}
					\|A(I-P_{B\cup V})\|_{p,2}\leq 2\poly(k) \min_{H\subseteq A-B, \dim(H)=k}\|A(I-P_{B\cup H})\|_{p,2}.
				\end{equation*}
			 Initialize $S=B.$\;
			\While {$|S-B|<O((20k/\epsilon)^p\cdot k^2/\epsilon\cdot\log(k/\epsilon))$}{
				 Pick $a_i$ according to:
				$
					P(\text{picking } a_i)\propto d(a_i, \text{span}(V\cup S)).
				$\;
				 $S\leftarrow S\cup\{a_i\}$.\;
			}
			\Return{ $S$.}
	\end{algorithm}
	
	The proof of the correctness of \fref{alg:samplingsubspace} is very similar to the proof in the original paper, except we start with a $\poly(k/\epsilon)$-approximation instead of an $O(1)$-approximation. We also need to carefully check that we can take the union with the ``base'' subspace $B$ without affecting the result. For completeness, we include the modified theorems here.
	\begin{lemma}[Modified Theorem 9 in \cite{deshpande2007sampling}]\label{lma:subspaceapproximation}
		Define
		\[
			H_k^* = \argmin_{H\subseteq A-B, H\ k\text{-dim}}\|A(I-P_{B\cup H})\|_{p,2}.
		\]
		Using a subspace $V$ of dimension at least $k$ such that
		\[
			(\sum_{i=1}^n d(a_i, V\cup B)^p)^{1/p}\leq 2\poly(k/\epsilon)(\sum_{i=1}^n d(a_i, H_k^*\cup B)^p)^{1/p},
		\]	
		\textsc{SamplingDimReduce} finds, with probability at least $1-(\epsilon/2k)^{2k^2/\epsilon}$, $S$ such that $\text{span}(V\cup B\cup H_S)$ contains a $k$-dimensional subspace $H'$ such that
		\[
			(\sum_{i=1}^n d(a_i, H'\cup B)^p)^{1/p}\leq (1+\epsilon)(\sum_{i=1}^n d(a_i, H_k^*\cup B)^p)^{1/p}.
		\]
	\end{lemma}
	
	To prove this lemma, we need the following two auxiliary lemmas from \cite{deshpande2007sampling}:
			\begin{lemma}[Lemma 12 in \cite{deshpande2007sampling}, proven in \cite{shyamalkumar2007efficient}]\label{lma:sinebetweenspaces}
		Let $F$ be a $k-$dimensional subspace in $\R^n$ for some $k>0$, $l'$ be any line, $\alpha(l')$ be the sine of the angle that $l'$ makes with $F$, $l$ the projection of $l'$ onto $F$ (if $\alpha(l')=1$ then take $l$ to be any line in $F$), $E$ the orthogonal complement of $l$ in $F$, and $\hat F$ the subspace spanned by $E$ and $l'$. Suppose that $a\in\R^n$ is such that $d(a, \hat F)>(1+\delta/2)d(a, F)$. Then there is a line $l''$ in the subspace spanned by $l'$ and $a$ such that $\alpha(l'')$, the sine of the angle made by $l''$ with $F$, is at most $(1-\delta/4)\alpha(l')$.
	\end{lemma}
	
	\begin{lemma}[Modified Lemma 10 in \cite{deshpande2007sampling}]\label{lma:probabilitygoodstep}
		Suppose that the our algorithm is in phase $j<k$. Then with probability at least $(\delta/10\poly(k))^p$, the point $a_i$ sampled in the step has the property that $d(a_i^\circ, \hat F^\circ)>(1+\delta/2)d(a_i^\circ, F_j^\circ)$. 
	\end{lemma}
	\begin{proof}
		We must have
		\[
			\p{\sum_i^n d(a_i, \hat F\cup B)^p}^{1/p}>(1+\delta)\p{\sum_i^n d(a_i,  F_j\cup B)^p}^{1/p}
		\]
		otherwise we would not be in phase $j$. We call a point $a_i$ a ``witness'' if
		\[
			d(a_i, \hat F)>(1+\delta/2)d(a_i, F_j).
		\]
		Let $W\subseteq [n]$ corresponds to the set of all ``witness'' points. We claim that
		\[
			\p{\sum_{i\in W}^n d(a_i, V\cup H_S\cup B)^p}^{1/p}>\frac{\delta}{10}\p{\sum_i^n d(a_i,  V\cup H_S\cup B)^p}^{1/p}.
		\]
		for the current sample $S$. That is, with probability at least $(\delta/10)^p$ our algorithm picks a ``witness'' point $a_i$ in the next step. Suppose this is not the case. Then let $h_i$ be the projection of $a_i$ onto span$(V\cup H_S\cup B)$.
		
		We have $d(a_i, \hat F)\leq (1+\delta/2)d(a_i, F_j)$ for $i\in[n]\backslash W$, and for $i\in W$, we have
		\begin{align*}
			d(a_i, \hat F)&\leq d(a_i, h_i)+d(h_i, \hat F)\\
			&\leq d(a_i, h_i)+d(h_i, F_j)\\
			&\leq 2d(a_i, h_i)+d(a_i, F_j)\\
			&\leq 2d(a_i, h_i)+\p{1+\delta/2}d(a_i, F_j).
		\end{align*}
		
		By Minkowski's inequality, we have
		\begingroup
		\allowdisplaybreaks
		\begin{align*}
			\p{\sum_i^n d(a_i, \hat F)^p}^{1/p}
			&\leq  \p{1+\delta/2}\p{\sum_i^n d(a_i, F_j)^p}^{1/p}+2\p{\sum_{i\in W}^n d(a_i, h_i)^p}^{1/p}\\
			&\leq \p{1+\delta/2}\p{\sum_i^n d(a_i, F_j)^p}^{1/p}+\frac{2\delta}{10\poly(k)}\p{\sum_{i=1}^n d(a_i, \spn(V\cup H_S\cup B))^p}^{1/p}\\
			&\leq \p{1+\delta/2}\p{\sum_i^n d(a_i, F_j)^p}^{1/p}+\frac{2\delta}{5}\p{\sum_{i=1}^n d(a_i, \spn(H^*_k\cup B))^p}^{1/p}\\
			&\leq \p{1+\delta}\p{\sum_i^n d(a_i, F_j)^p}^{1/p},
		\end{align*}
		\endgroup
		which is a contradiction to our assumption that this is in phase $j$.
		
		Hence with probability at least $(\delta/10\poly(k))^p$, the point $a_i$ picked in the next step is a ``witness'' point. This means that
		\begin{align*}
			d(a_i^\circ, \hat F^\circ)&=d(a_i, \hat F)\\
			&>\p{1+\frac{\delta}{2}d(a_i, F_j)}\\
			&=\p{1+\frac{\delta}{2}d(a_i^\circ, F_j^\circ)}.\qedhere
		\end{align*}
	\end{proof}
	
	We are now ready to prove \cref{lma:subspaceapproximation}.
	\begin{proof}[Proof of \cref{lma:subspaceapproximation}]
		Let $\delta = \frac{\epsilon }{2k}$. Let phase $j$ for some $0\leq j\leq k$ be such that for the current sample $S$, there is a $k$-dimensional subspace $F_j$ such that $\dim(F_j\cap \text{span}(V\cup H_S))\geq j$ and
		\[
			\p{\sum_{i=1}^n d(a_i, F_j\cup B)^p}^{1/p}\leq (1+\delta)^j\p{\sum_{i=1}^n d(a_i, H_k^*\cup B)^p}^{1/p}.
		\]
		
		Once we enter phase $j$, all the following steps will be in phase at least $j$. Reaching phase $k$ means we are done since we then find $F_k\subseteq \text{span}(V\cup H_S)$ and
		\[
			\p{\sum_{i=1}^n d(a_i, F_k\cup B)^p}^{1/p}\leq (1+\delta)^k\p{\sum_{i=1}^n d(a_i, H_k^*\cup B)^p}^{1/p} \leq (1+\epsilon)\p{\sum_{i=1}^n d(a_i, H_k^*\cup B)^p}^{1/p}.
		\]
		At the beginning we start with $\dim(V\cup H_k^*)=j$ and $F_j=H_k^*$.
		
		When we are about to execute the first step in phase $j$, let $G=\spn(F_j\cup B)\cap \spn(H_k^*\cup B)$. Let $\dim(B)=b$. Then $G$ is a $(j+b)$-dim subspace. Let $F_j^\circ$ and $V^\circ$ be the orthogonal complement of $G$ in $F_j\cup B$ and $\spn(V\cup B\cup H_S)$ respectively. Note that $B\subseteq G$, so our notation makes sense here. Let $l$ be a line in $F_j^\circ$ that makes the smallest angle with $V^\circ$ and $l^\circ$ a line in $V^\circ$ that makes this angle with $l$. This angle must be bigger than $0$ since otherwise we will be executing a phase $j'>j$. Let $\hat F^\circ$ be the rotation of $F_j^\circ$ to contain $l^\circ$, and let $\hat F$ be the $k$-dimensional subspace given by $\spn(\hat F^\circ\cup G-B)$. Note that $\dim(\hat F\cap\spn(V\cup H_S))=j'>j$. If $\p{\sum_{i=1}^n d(a_i, \hat F\cup B)^p}^{1/p}\leq (1+\delta)\p{\sum_{i=1}^n d(a_i, F_j\cup B)^p}^{1/p}$, then we execute in phase $j'$ with $F_{j'}=\hat F$.
		
		Otherwise we execute after more than one step in phase $j$ and we added a few dimensions to obtain a new $\spn(V\cup H_S)$. Let $l$ be a line in $F_j^\circ$ that is closest to the new $V^\circ$, i.e., the orthogonal complement of the old $G$ in the new $\spn(V\cup H_S)$. Let $l^\circ$ be a line in $C^\circ$ that makes the smallest angle with $l$, and let $\alpha_j'$ be the sine between $l$ and $l^\circ$. There are several cases:
		\begin{enumerate}
			\item $\alpha_j'=0$. Then $\dim(F_j\cap\spn(V\cup H_S))=j'>j$ and we will execute in phase $j'$ with $F_{j'}=F_j$.
			\item $\alpha_j'>0$. Let $\hat F^\circ$ be the rotation of $F_j^\circ$ that contains $l^\circ$, and $hat F$ be the $k-$dimensional subspace given by $\spn(\hat F^\circ\cup G-B)$.
				\begin{enumerate}
					\item If it is the case that
						\begin{equation*}
							\p{\sum_{i=1}^n d(a_i, \hat F\cup B)^p}^{1/p}\leq (1+\delta)\p{\sum_{i=1}^n d(a_i, F_j\cup B)^p}^{1/p},
						\end{equation*}
						we execute in phase $j'>j$ such that $F_{j'}=\hat F$.
					\item 
						Otherwise we execute the next step in phase $j$.
				\end{enumerate}
		\end{enumerate}
		Once we attempt to execute a step in phase $k$, then all subsequent steps will simply execute in phase $k$. Thus we have completely classified all the steps of our algorithm into $(k + 1)$ phases. Now we will show that the algorithm succeeds, i.e., it executes some step in phase $k$, with high probability. To do this, we need to show that each phase contains only a few steps. Let us call a step of the algorithm good if (i) either the step executes in phase $k$, or (ii) the step executes in some phase $j < k$ and the point $a_i$ sampled in the step has the property that $d(a_i^\circ, \hat F^\circ)>(1+\delta/2)d(a_i^\circ, F_j^\circ)$, where for any point $a_i$, $a_i^\circ$ is the projection of $a_i$ into the orthogonal complement of $G$.
		
		Consider some phase $j < k$ in which we execute one or more steps. We bound the number of good steps in phase $j$. Let us use $\alpha_j$ to denote the sine of the angle between $l$ and $l^\circ$ before the execution of the first step in the phase, and $\alpha_j'$ to denote the same quantity at any subsequent point in the phase. We first bound $\alpha_j$. Let $\bar a_i$ denote the projection of $a_i$ onto $F_j\cup B$, and $\bar a_i^\circ$ denote the projection of $\bar a_i$ onto the orthogonal complement of $G$. Focusing on the beginning of phase $j$, we have
		\begingroup
		\allowdisplaybreaks
		\begin{align}
			\alpha_j\p{\sum_{i}^n \|\bar a_i^\circ\|^p}^{1/p}
			&\leq \p{\sum_i^n d(\bar a_i^\circ, V^\circ)^p}^{1/p} \nonumber\\
			&=\p{\sum_i^n d(\bar a_i, \spn(V\cup B\cup H_S))^p}^{1/p} \nonumber\\
			&\leq \p{\sum_i^n d(\bar a_i, a_i)}^{1/p}+\p{\sum_i^n d( a_i, \spn(V\cup B\cup H_S))^p}^{1/p} \nonumber\\
			&=\p{\sum_i^n d(\bar a_i, F_j\cup B)}^{1/p}+\p{\sum_i^n d( a_i, \spn(V\cup B\cup H_S))^p}^{1/p} \nonumber\\
			&\leq  \p{\poly(k)+(1+\delta)^j}\p{\sum_i^n d(\bar a_i, H_k^*\cup B)}^{1/p} \nonumber\\
			&\leq 2\poly(k)\p{\sum_i^n d(\bar a_i, H_k^*\cup B)}^{1/p}.\label{eq:1}
		\end{align}
		\endgroup
		where the second to last inequality was because $\delta<1/2k$ and our initial assumption about $V$.
		If a step in phase $j$ is good, then by Lemma~\ref{lma:sinebetweenspaces}, there is a line in span$(a_i^\circ, l^\circ)$ for which the sine of its angle with $F_j^\circ$ is at most $(1-\delta/4)$ times the value of $\alpha_j'$ before the step.
		Taking $O(1/\delta\log \poly(k)/\delta)$ good steps in phase $j$, then after these steps we have $\alpha_j'\leq (\delta/8\poly(k))\alpha_j$. Hence
		\begingroup
		\allowdisplaybreaks
		\begin{align*}
			\p{\sum_i^n d(a_i, \hat F\cup B)^p}^{1/p}
			&\leq  \p{\sum_i^n d(a_i,\bar a_i)^p}^{1/p}+\p{\sum_i^n d(\bar a_i, \hat F\cup B)^p}^{1/p}\\
			&\leq  \p{\sum_i^n d(a_i,F_j\cup B)^p}^{1/p}+\p{\sum_i^n d(\bar a_i, \hat F\cup B)^p}^{1/p}\\
			&\leq  \p{\sum_i^n d(a_i,F_j\cup B)^p}^{1/p}+\p{\sum_i^n d(\bar a_i^\circ, \hat F^\circ)^p}^{1/p}\\ 
			&\leq \p{\sum_i^n d(a_i,F_j\cup B)^p}^{1/p}+\alpha_j'\p{\sum_{i}^n \|\bar a_i^\circ\|^p}^{1/p}\\
			&\leq  \p{\sum_i^n d(a_i,F_j\cup B)^p}^{1/p}+\frac{\delta}{8\poly(k)}\alpha_j\p{\sum_{i}^n \|\bar a_i^\circ\|^p}^{1/p}\\
			&\leq (1+\delta)\p{\sum_i^n d(a_i,F_j\cup B)^p}^{1/p}.
		\end{align*} 
		\endgroup
		where the last step is from equation~\ref{eq:1}. This says that we have reached phase $j'>j$. 
		\textsc{SamplingDimReduce} runs  $N=O((\poly(k)/\delta)^p\cdot k/\delta\cdot \log(\poly(k)/\delta))$ steps. Failing to reach phase $k$ means it encounters fewer than $O(k/\delta\log \poly(k)/\delta)$ good steps. From Lemma~\ref{lma:probabilitygoodstep}, we have that a step is good with probability at least $(\delta/10\poly(k))^p$. Thus the probability that the algorithm fails to reach phase $k$ in $N$ steps is bounded by $\delta^{k/\delta}$.
		
		Thus with probability at least $1-\delta^{k/\delta}$, in the end the span$(V\cup H_S)$ contains a subspace $H'$ of dimension $k$ such that
		\[
				\p{\sum_{i=1}^n d(a_i, H'\cup B)^p}^{1/p}\leq (1+\delta)^k\p{\sum_{i=1}^n d(a_i, H_k^*\cup B)^p}^{1/p} \leq (1+\epsilon)\p{\sum_{i=1}^n d(a_i, H_k^*\cup B)^p}^{1/p}. \qedhere
		\]
	\end{proof}

	For our coreset construction, we follow the same procedure in \cref{sec:mainsparse}, but here we sample the subspace iteratively.
	
	\IncMargin{1em}
	\begin{algorithm}[!ht]
		\DontPrintSemicolon
	    \SetKwInOut{Input}{Input}
	    \SetKwInOut{Output}{Output}
	    \SetKwData{Start}{start}
	    \SetKwData{End}{end}
		\caption{\textsc{SamplingDimensionReduction}}\label{alg:samplingdimensionreduction}
			\Input{ $A\in\R^{n\times d}$, $k, \epsilon>0$}
			\Output{ Projection matrix $P_S = WW^T$ with $W \in \mathbb{R}^{d \times d_W}$ where $\mathbb E[d_W] = \poly(k/\epsilon)$}
			 $\tau \leftarrow \Theta(\epsilon^{2/p})$.\;
			 $i^* \leftarrow $ uniformly random integer from $[10/\tau]$.\;
			 Initialize $W_1\leftarrow \emptyset$, $P_S \leftarrow 0$.\;
			\For {\texttt{$i=0; i<i^*; i=i+1$}} {
			     $P_{\hat{X}}(= WW^T) \leftarrow$ \fref{alg:polykapprox}$(A,P_S,k,\epsilon)$.\;
				 $P_{S'}(= UU^T) \leftarrow$ \fref{alg:samplingsubspace}$(A,P_S,k,P_{\hat{X}},\epsilon,\poly(k/\epsilon))$.\;
				 $W_1 \leftarrow [W_1 | U ]$.\;
				 $P_S(=W_1W_1^T) \leftarrow P_S + P_{S'}$.\;
			}
			\Return{ $P_S(=W_1W_1^T).$}
	\end{algorithm}
	\DecMargin{1em}
	
	\IncMargin{1em}
	\begin{algorithm}[!ht]
			\DontPrintSemicolon
	    \SetKwInOut{Input}{Input}
	    \SetKwInOut{Output}{Output}
	    \SetKwData{Start}{start}
	    \SetKwData{End}{end}
	\caption{\textsc{SamplingCoresetsConstruction}}
	 \label{alg:samplingcoreset}
	\Input{ $A \in \mathbb{R}^{n \times d}$, $k,\epsilon>0$.}
	\Output{ $\epsilon$-strong coreset $B$.}
	 Let $P_S=$\fref{alg:samplingdimensionreduction}$(A,  k, \epsilon)$.\;
	 Let $v\in\R^d$ be an all $0$ vector.\;
	\For{$i=1,\ldots,n$}{
	     Let $v_i$ be a $(1+\epsilon)$-approximation to $\|A_i(I-P_S)\|_2$. Using the algorithm in \cite{clarkson2017low}, each regression problem succeeds with probability at least $1-\frac{1}{n^2}$.\;
	}
		Construct a strong coreset $B$ using \cite{sohler2018strong} on $[AP_S, v].$\;
	\Return{$B$.}
	\end{algorithm}

	\DecMargin{1em}
	
		Using \fref{alg:samplingdimensionreduction}, we obtain the following strong coresets for subspace approximation and $k$-Median.	
			
	\begin{theorem}[Strong coresets for subspace approximation, modified Theorem 17 in \cite{sohler2018strong}, $p>2$]\label{thm:samplingcoresetsubspaceapprox}
		For $p>2$, there exists $TB\in\R^{\poly(k/\epsilon)\times d+1}$ such that for any $\rank-k$ orthogonal projection $P$, we have:
		\[
			|{\|A-AP\|_{p,2}^p-\|TB-(TB_{-1}P)_{+1}\|_{p,2}^p}|\leq\epsilon \|A-AP\|_{p,2}^p
		\]
		We can find such a $TB$ in $\widetilde O(nd\poly(k/\epsilon))$ time. 
	\end{theorem} 
	\begin{proof}
		The correctness of the statement is proven in Theorem~\ref{thm:coresetsubspaceapprox} and \cite{sohler2018strong}. The time complexity follows from the original proof and the time complexity of \fref{alg:samplingcoreset}.
	\end{proof}
		
	\begin{theorem}[Strong coresets for $k$-median, modified Theorem 18 in \cite{sohler2018strong}]\label{thm:samplingcoresetkmedian}
		Using same notations in \cref{thm:coresetkmedian}. Let $\epsilon\in(0,1]$. Given a matrix $A\in\R^{n\times d}$, \fref{alg:samplingcoreset} compute in time $ \widetilde O(nd\poly(k/\epsilon))$ a matrix $B\in\R^{s\times (d+1)}$ where $s=O(\frac{\poly(k/\epsilon)k^2\log k}{\epsilon^2})$ and non-negative weights $w_1,\ldots, w_s$ such that with probability at least $3/5$ for every set $C$ of $k$ centers, we have
		\[
			|\|A-A^C\|_{p,2}^p-\sum_{i\in[s]}w_i\|S_{i*}-S_{i*}^C\|_2^p|\leq\epsilon\|A-A^C\|_{p,2}^p.
		\]
	\end{theorem}
	
	\begin{proof}
		As proven in \cite{deshpande2007sampling}, one iteration of \textsc{SamplingDimReduce} runs in time $O(nd\poly(k/\epsilon))$. Since we run $\Theta(1/\epsilon^{2/p})$ times, in total it results in $O(nd\poly(k/\epsilon))$ time.  
		The subspace $S$ returned by \fref{alg:samplingdimensionreduction} satisfies Lemma~\ref{lma:meetsallconditions}, so the correctness of the statement follows from Theorem~\ref{thm:coresetkmedian}.
	\end{proof}
