# Supplementary material for: Dimensionality Reduction for Sum-of-Distances Metric
Source: arXiv:1912.12003 source file (2021-06-24)
Supplement: Supplementary file 3 [file appendix_sparse.tex]

 \section{Proofs of Strong Coreset Construction}\label{sec:coreset_appendix}

	Given the desired subspace $S$ in \cref{lma:meetsallconditions}, one of the steps is to calculate $AP_S$, but this is too expensive. \cite{sohler2018strong} provides a way to efficiently approximate this value, but the original proof has a minor error. We state the original lemma and the corrected proof here as well.
	\begin{lemma}[Lemma 14 in \cite{sohler2018strong}]\label{lma:sohlerlma14}
		Given $S$, the subspace guaranteed by Lemma~\ref{lma:meetsallconditions}, we can compute in time $O(\nnz(A)\log n+(n+d)\cdot\poly(k/\epsilon))$ a matrix $\widetilde B$ of rank $\poly(k/\epsilon)$ such that with probability at least $9/10$ we have for every set $C$ contained in a $k$-dimensional subspace
		$
			|\|B-B'\|_{p,2}^p-\|\widetilde B-\widetilde B'\|_{p,2}^p|\leq\epsilon\|A-A'\|_{p,2}^p.
		$
	Here $B'$ and $\widetilde{B'}$ are the matrices that contain in the $i$-th row in the first $d$ coordinates the point from (the closure of) $C$ that is closest to the $i$-th row of $B_{-1}$ and $\widetilde{B}_{-1}$ respectively and have $d+1$-st coordinate $0$.
	\end{lemma}
	\begin{proof}
		The original proof in \cite{sohler2018strong} (proof of Lemma 14) had a minor error in Equation (2). We present here how to get the same requirement of Equation (2) in their paper.
		
		Let $P = VV^T$ be the orthogonal projection onto $S$. Instead of computing the product $AP$, we solve the regression problems
		\begin{equation}
		    \min_x \|Vx - A_i^T\|_2
		\end{equation}
		and then obtain $\widetilde{A}_i = X_iV^T$ where $X_i^T$ is an approximate solution to the above regression problem for all values of $i$. We run the algorithm of \cite{polynomial-kernel} (see also Section 2.3 of \cite{dw-sketching}) which gives us $X_i$ for all values of $i$ given by 
		\begin{equation*}
		    X_i = A_iR^T[(RV)^-]^T
		\end{equation*}
		in time $O(\nnz(A)\log(n) + (n+d)\log(n)\poly(k/\epsilon))$ where $R$ is a Count-Sketch matrix with $O(\poly(k/\epsilon) \cdot \log(n))$ rows ($R$ maybe different for different values of $i$. But there are only $O(\log n)$ distinct $R's$ used by the algorithm) such that with probability $9/10$, for all values of $i$, $R$ obtained for that particular $i$ is a subspace embedding for $[V\ A_i^T]$ and 
		\begin{equation*}
		    \|VX_i^T - V(X_i^*)^T\|_2 \le O(\epsilon)\text{OPT}_i \quad
		\end{equation*}
		where 
		\begin{equation*}
		    (X_i^*)^T = \text{argmin}_x \|Vx - A_i^T\|_2 = V^TA_i^T
		\end{equation*}
		and 
		\begin{equation*}
		    \text{OPT}_i = \|VV^TA_i^T-A_i^T\|_2 = \|A_i - A_iVV^T\|_2 = \|A_i - A_iP\|_2.
		\end{equation*}
		See \cite{sarlos-random-projection}, which gives the above guarantee for any subspace embedding.
		
		Hence, we obtain
		\begin{equation*}
		    \|\widetilde{A}_i - A_iP\|_2 = \|\widetilde{A}_i - A_iVV^T\|_2 = \|X_iV^T - X_i^*V^T\|_2 \le O(\epsilon)\|A_i-A_iP\|_2.
		\end{equation*}
		From here, the proof proceeds as is in the proof of Lemma 14 in \cite{sohler2018strong}.
	\end{proof}

	\subsection{Strong Coreset for Subspace Approximation}
	For the proof of a coreset construction for subspace approximation, we state the following lemma:
	\begin{lemma}[Lemma 16 in \cite{sohler2018strong}]\label{lma:lma16insohler}
		Given $S$, let $B=[AP_S, v]$ where $v_i=(1\pm\epsilon)\|A_{i*}-(AP_S)_{i*}\|$. Then in $n\cdot \poly(k\log n/\epsilon)$ time it is possible to find a sampling and rescaling matrix $T$ with $O(\poly(\rank(S)/\epsilon))$ rows for which for all rank-$k$ orthogonal projection matrices $P$:
		\[
			\|T B-(T B_{-1} P)_{+1}\|_{p,2}^p=(1 \pm \epsilon)\|B-(B_{-1} P) _{+1}\|_{p,2}^p.
		\] 
		Letting $S$ be the output of Algorithm~\ref{alg:coreset}, $T$ would have $O(\poly(k/\epsilon))$ rows.
	\end{lemma}
	
		\begin{proof}[Proof of \cref{thm:coresetsubspaceapprox}]
		Let $B$ be the output of Algorithm~\ref{alg:coreset}. We represent $B=[AP_S,  v]$, where $P_S$ is the projection onto $S$ and it is given in the form $P_S=UU^T$, and $v_i=(1\pm\epsilon)\|A_{i*}-A'_{i*}\|_2$, $A'=AP_S$ for $i\in[n]$.
		
		By Lemma~\ref{lma:meetsallconditions}, we obtain (see Remark 7 in \cite{sohler2018strong} for detail)
		\[
			|\|A-A P\|_{p, 2}^{p}-\|B-(B_{-1} P )_{+1}\|_{p, 2}^{p} | \leq \epsilon\|A-A P\|_{p, 2}^{p}
		\] 
		By Lemma~\ref{lma:lma16insohler}, we can find a sampling and rescaling matrix $T$ such that for all rank-$k$ orthogonal projections $P$, $\left\|T B-(T B_{-1} P) _{+1}\right\|_{p, 2}^{p}=(1 \pm \epsilon)\left\|B-(B_{-1} P )_{+1}\right\|_{p, 2}^{p}$. Therefore:
		\[
			\begin{aligned}|\| A-A P\|_{p, 2}^{p}-\| T B-(T B_{-1} P) _{+1} \|_{p, 2}^{p} | &=|\|A-A P\|_{p, 2}^{p}-\|B-(B_{-1} P)_{+1}\|_{p, 2}^{p} | \pm \epsilon\|B-(B_{-1} P) _{+1}\|_{p, 2}^{p} \\ 
			& \leq \epsilon\|A-A P\|_{p, 2}^{p}+\epsilon\|B-(B_{-1} P) _{+1}\|_{p, 2}^{p} \\ 
			& \leq \epsilon\|A-A P\|_{p, 2}^{p}+\epsilon(\|A-A P\|_{p, 2}^{p}+\epsilon\|A-A P\|_{p, 2}^{p}) \\ 
			& \leq(2 \epsilon+\epsilon^{2})\|A-A P\|_{p, 2}^{p} \end{aligned}
		\]
		For the time complexity, Algorithm~\ref{alg:coreset} outputs s in $\widetilde O(\nnz(A)/\epsilon+(n+d)\poly(k/\epsilon))$ time. By Lemma~\ref{lma:lma16insohler}, $T$ is found in $n\poly(k\log n/\epsilon)$ time. $T$ selects $\poly(k/\epsilon)$ rows of $A$, and for each we project onto $S$, which takes $d\poly(k/\epsilon)$ time in total. The construction of the coreset $TB$ then yields the claimed running time.
	\end{proof}
	
	\subsection{Strong Coreset for \texorpdfstring{$k$}{k}-Median}
	
	We remark that Algorithm~\ref{alg:coreset} satisfies:
	\begin{theorem}[Theorem 8 in \cite{sohler2018strong}]\label{thm:sohlerthm8}
		Let $\epsilon\in(0,1]$. Let $A\in\R^{n\times d}$ be the input matrix, $B\in\R^{n\times (d+1)}$ be the rank $\poly(k/\epsilon)$ matrix output by \textsc{CoresetConstruction}. Let $c\in\R^d$ be any non-empty set that is contained in a $k$-dimensional subspace. Let $A'$ and $B'$ be the matrices whose rows are the closest points in the closure of $C$ with respect to the rows of $A$ and $B_{-1}$ respectively. Then we have
		$
			\abs{\|A-A'\|_{1,2}-\|B-B'_{+1}\|_{1,2}}\leq\epsilon\|A-A'\|_{1,2}.
		$
	\end{theorem}
		\begin{proof}[Proof of \cref{thm:coresetkmedian}]
		This proof is essentially the same as the proof in \cite{sohler2018strong}, except we need to change the running time and coreset size carefully.
		
		With $\epsilon/10$, $T$ returned by Algorithm~\ref{alg:dimensionreduction} satisfies Lemma~\ref{lma:meetsallconditions} with probability at least $9/10$. $T$ has rank $\poly(k/\epsilon)$ and can be computed in $O(\nnz(A)/\epsilon+(n+d)\poly(k/\epsilon))$. By Lemma~\ref{lma:sohlerlma14}, with probability at least $9/10$, we compute $\widetilde B$ of rank $\poly(k/\epsilon)$ in time $O(\nnz(A)\log n+(n+d)\poly(k/\epsilon))$. 
		
		Using the coreset construction in \cite{braverman2016new,feldman2011unified}, in time $\widetilde O\p{n\poly\p{\frac{k\log(1/\delta)}{\epsilon}}}$ we obtain a coreset $S^*$ of size $O(\frac{\poly(k/\epsilon)k^2\log k}{\epsilon^2})=\poly(k/\epsilon)$. For each point in $S^*$, we calculate its coordinates in the original space, which takes $O(d\poly(k/\epsilon))$ time.
		
		\cref{lma:sohlerlma14} and \cref{thm:sohlerthm8} guarantee the following:
		\begin{align*}
			&|{\|B-B'_{+1}\|_{1,2}-\|\widetilde B-\widetilde B'\|_{1,2}}|\leq\epsilon\|A-A'\|_{1,2}\\
			&\abs{\|A-A'\|_{1,2}-\|B-B'_{+1}\|_{1,2}}\leq\epsilon\|A-A'\|_{1,2}.
		\end{align*}
		Here $\widetilde{B'}$ is the matrix that contains in the $i$th row in the first $d$ coordinates the point from (the closure of) $C$ that is closest to the $i$-th row of $\widetilde{B}_{-1}$ respectively and have $(d+1)$th coordinate $0$.
		By the definition of coresets $S$ we also have:
		\[
			|{\|\widetilde B-\widetilde B'\|_{1,2}-\sum_{i\in[|S|]}w_i\|S_{i^*}-S_{i*}^C\|_{1,2}}|\leq \epsilon \|\widetilde B-\widetilde B'\|_{1,2}.
		\]
		These three inequalities imply:
		\begin{align*}
			&| \|A-A'\|_{1,2}- \sum_{i\in[|S|]}w_i\|S_{i^*}-S_{i*}^C\|_{1,2}  | \\
			&\leq 2\epsilon \|A-A'\|_{1,2}+\epsilon \|\widetilde B-\widetilde B'\|_{1,2}\\
			 &\leq 2\epsilon \|A-A'\|_{1,2}+\epsilon(1+2\epsilon)\|A-A'\|_{1,2}\\
			 &\leq 5\epsilon \|A-A'\|_{1,2}
		\end{align*}
		as desired.		
	\end{proof}
